# Supplementary material for: Solvothermal vapor annealing and environmental control setup with adjustable magnetic field module for GISAXS studies
Source: arXiv:2602.12086 ancillary file (2026-02-12)

# Supplementary Material

Solvothermal vapour annealing and environmental control setup  
with adjustable magnetic field module for GISAXS studies

## Contents

|                                                               |    |
|---------------------------------------------------------------|----|
| Figure S1: GISAXS schematic .....                             | 2  |
| Figure S2: Gauss probe and magnetic shelf geometries .....    | 2  |
| Figure S3: Sample stage patterning.....                       | 5  |
| Figure S4: TEM of maghemite nanoparticles.....                | 6  |
| Figure S5: Optical microscopy of embedded nanoparticles ..... | 7  |
| Figure S6: AFM on PS(38)- <i>b</i> -PF2MS(11) .....           | 10 |
| Figure S7: AFM on PS(21.7)- <i>b</i> -PB(60) .....            | 12 |

Christian Kjeldbjerg Kristensen, Bo Jakobsen, Miriam Varón,  
Kim Lefmann, Cathrine Frandsen, Dorte Posselt

**Figure S1: GISAXS schematic**

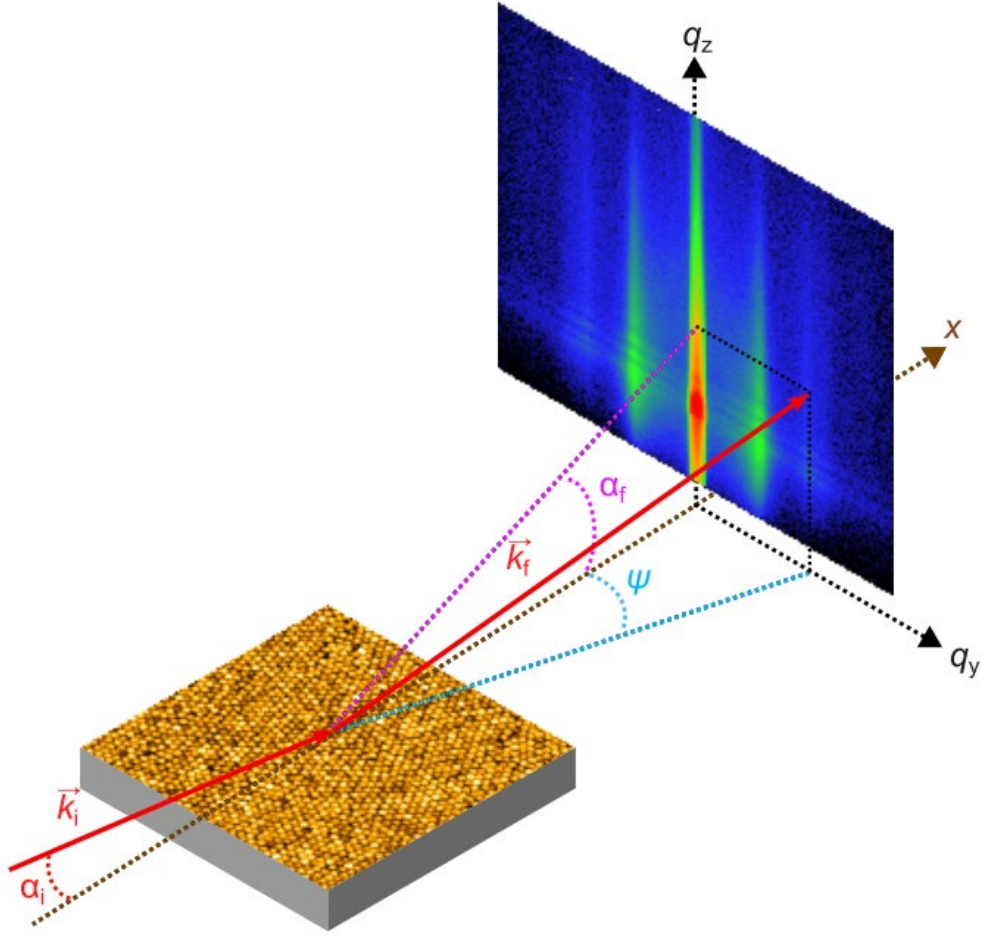

The diagram shows the grazing-incidence geometry used for GISAXS in this work. The incident plane wave has a wave-vector  $\vec{k}_i$  and impinges on the sample surface at the grazing angle  $\alpha_i$ . The surface-parallel x-axis is defined along the projection of  $\vec{k}_i$  onto the sample surface plane. The scattered wave has wave-vector  $\vec{k}_f$  and exits at the grazing angle  $\alpha_f$  in the plane defined by  $\vec{k}_i$  and the x-axis and at the in-plane azimuthal angle  $\psi$ , measured between the projection of  $\vec{k}_f$  and the x-axis. The scattering vector (momentum transfer)  $\vec{q} = \vec{k}_f - \vec{k}_i$  therefore has components

$$q_x = \frac{2\pi}{\lambda} (\cos \alpha_f \cos \psi - \cos \alpha_i), \quad q_y = \frac{2\pi}{\lambda} \cos \alpha_f \sin \psi, \quad q_z = \frac{2\pi}{\lambda} (\sin \alpha_f + \sin \alpha_i)$$

which map to the horizontal ( $q_y$ ) and vertical ( $q_z$ ) detector coordinates, respectively. The longitudinal component  $q_x$  is negligible in GISAXS geometry. Finally, we note that  $|\vec{k}_f| = |\vec{k}_i| = 2\pi/\lambda$ .

**Figure S2: Gauss probe and magnetic drawer setup**

a) Setup for Gauss probe measurements. The probe is secured with a clamp on a retort stand and the magnetic drawer is placed between two marked positions on the stand base to ensure consistent measurements.

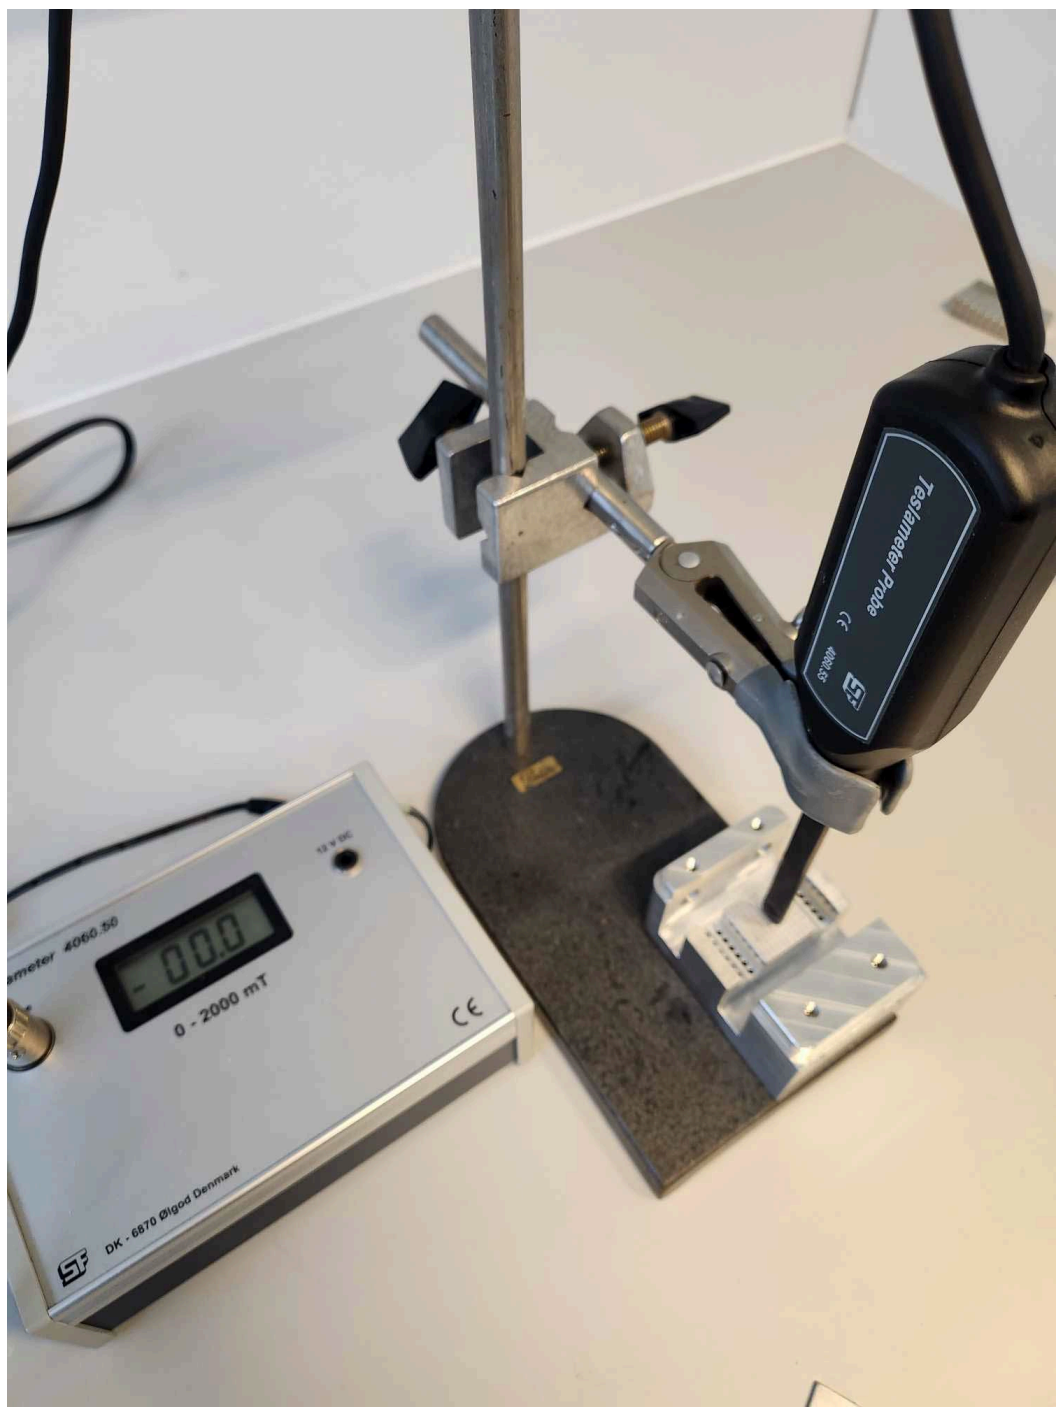

b) Schematic overview of the three orthogonal magnetic field geometries achievable with commercially available permanent magnets inserted into slots in the magnetic STVA drawer. The figure is arranged as two horizontal panels corresponding to two different viewing directions. The five illustrations of the setup in the upper panel are linked to the corresponding illustrations in the blower panel. In each panel the first image defines the viewing direction: is in the upper panel the in-plane axes have x pointing north and y east, while in the lower panel y is kept east but the viewing frame is rotated with z pointing north. The second image marked Schematic depicts the mechanical clearance around the sample table and marked with light-blue - volumes of  $10 \times 30 \times 50 \text{ mm}^3$  located on either side of the grey sample table, with an area of  $22 \times 22 \text{ mm}^2$ . The yellow square indicates the position of a  $10 \times 10 \text{ mm}^2$  sample on the sample table. A 1 cm scale bar provides dimensional reference. The remaining three images in each panel show the magnet layouts required to generate magnetic field directions along the x, z, or y direction marked x-config., z-config. and y-config., respectively. For the x- and z-config. stacks of  $10 \times 30 \times 5 \text{ mm}^3$  NdFeB bars are oriented with their poles opposite to the field generated between them; for the y-field case the bars lie face to back such as to generate a field in the gap between them. Green and red colours distinguish the two pole faces, while the absolute polarity is left unspecified. In the schematic for the y-config the scale of the magnets has been blown up for clarity.

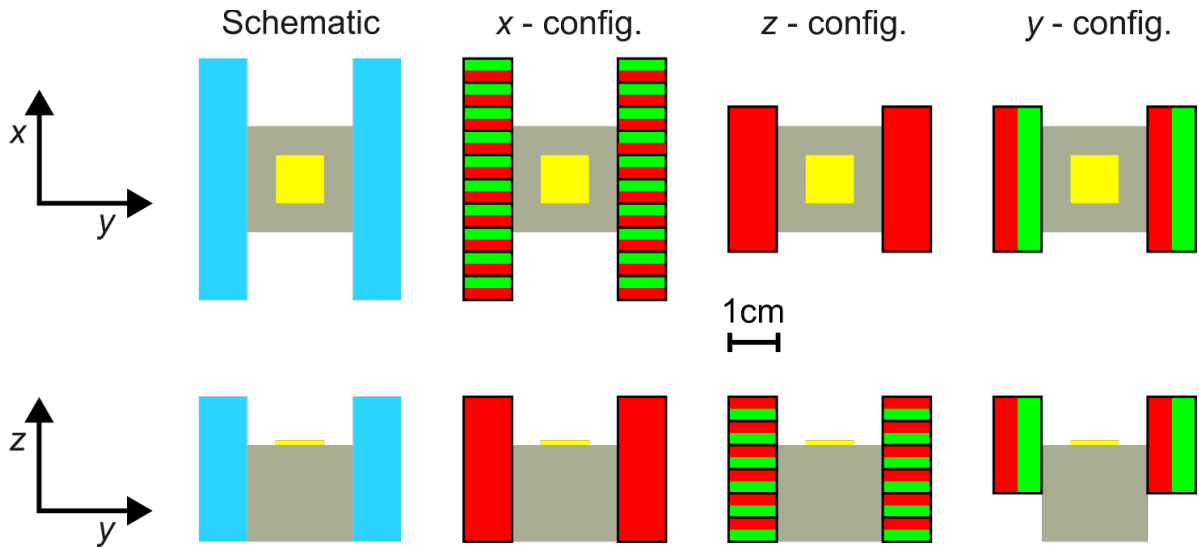

c) Finite elements simulations showing the magnetic field strength distribution at the position of the sample table. The top panel from left to right show the resulting field strength distribution as the arrays on each side of the sample are filled with 1, 2, 3, 4 and 5 bar magnets, respectively while the bottom panel from left to right show the magnetic field strength distribution after insertion of 6, 7, 8, 9, and 10 bar magnets, respectively. The colour scale has

been limited to 0.3 mT to ensure spatial inhomogeneities are clearly represented.

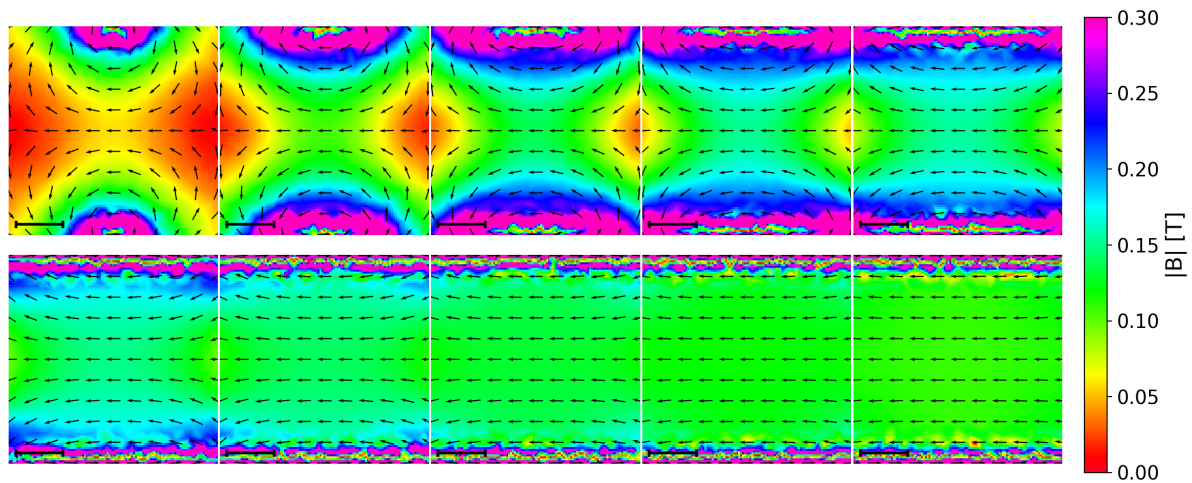

**Figure S3: Sample table patterning**

Magnetic drawer sample table (left) and post (right) patterning of the sample table.

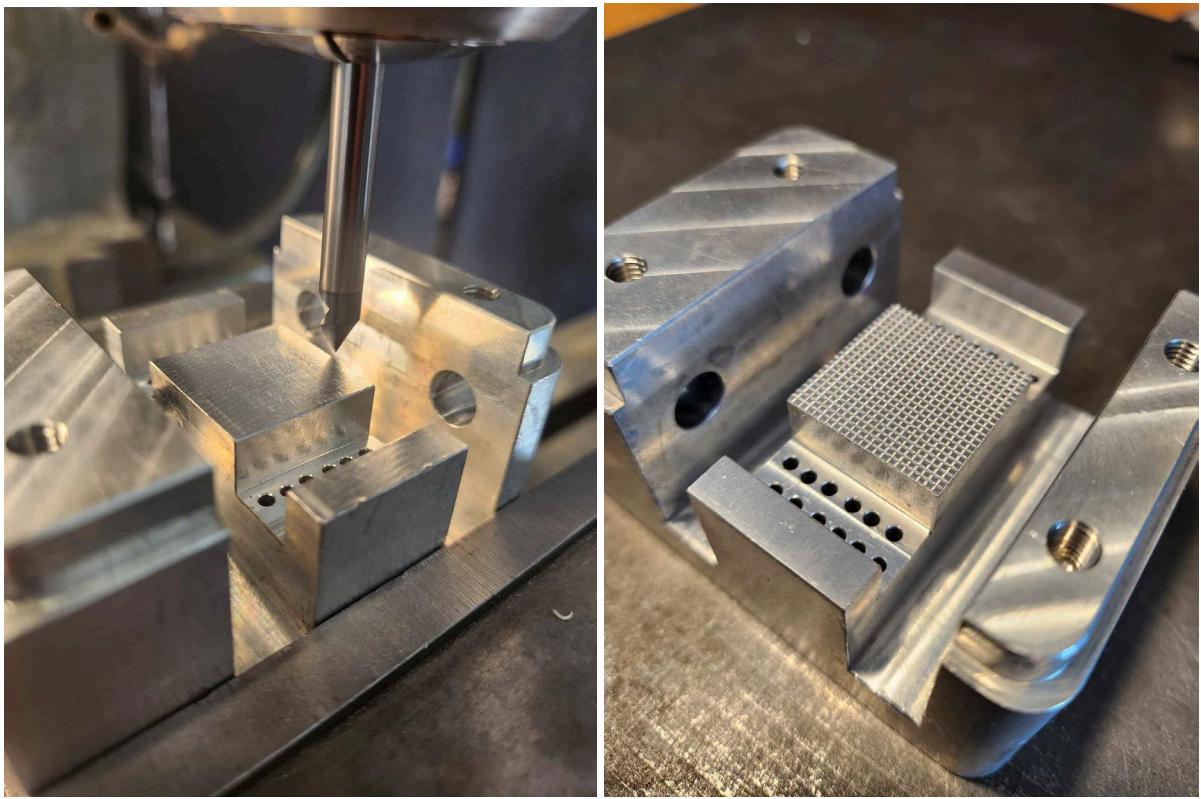

#### Figure S4: TEM of maghemite nanoparticles

a) Transmission electron microscopy (TEM) image of magnetic maghemite nanoparticles prior to coating. The histogram shows the nanoparticle size averaged over several TEM images.

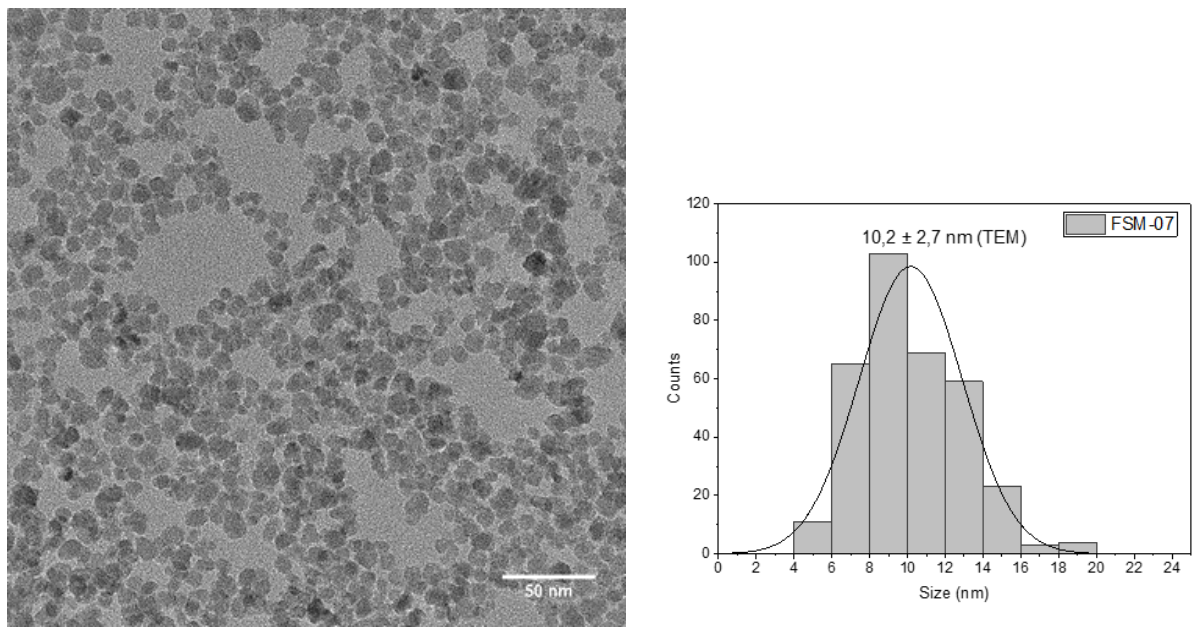

b) TEM images of nanoparticles after coating with polystyrene lithium poly(styrene sulfonate) (PSS-Li),  $M_n \approx 5$  kDa obtained from Polymer Standard Service GmbH.

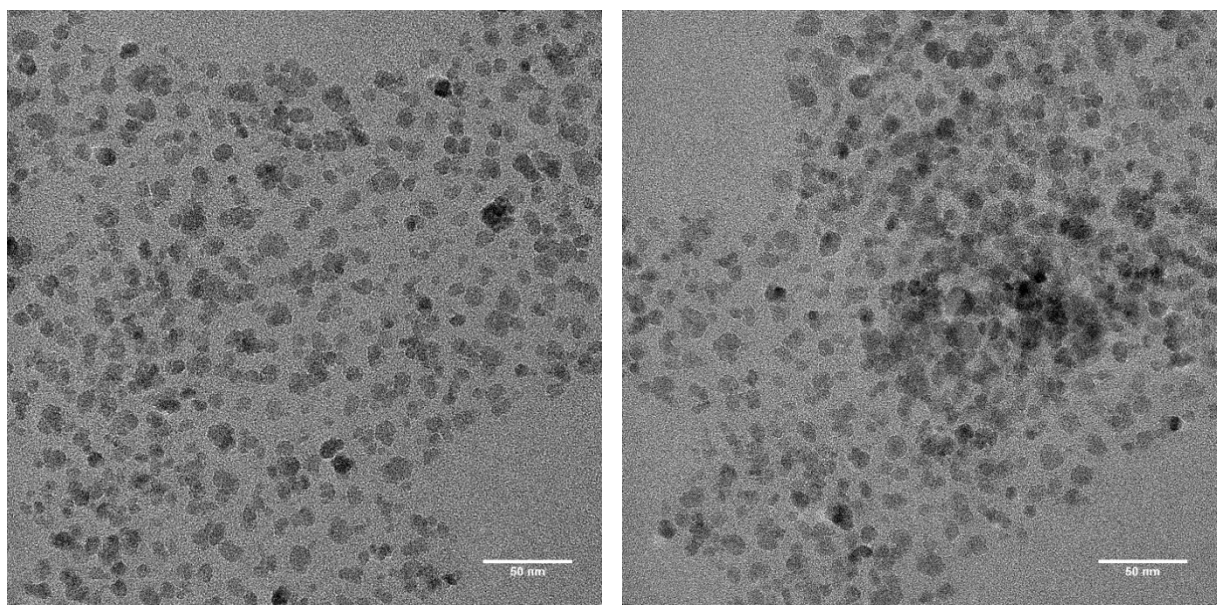

### Figure S5: Optical microscopy of nanoparticles

a) Optical microscopy image of polystyrene coated magnetic nanoparticle in polystyrene-*b*-polybutadiene matrix formed after solution coating onto a Si wafer in the STVA environmental chamber with a toluene saturated nitrogen atmosphere during drying and with the full array of permanent magnets installed inside the STVA chamber. Inset represents 100 microns.

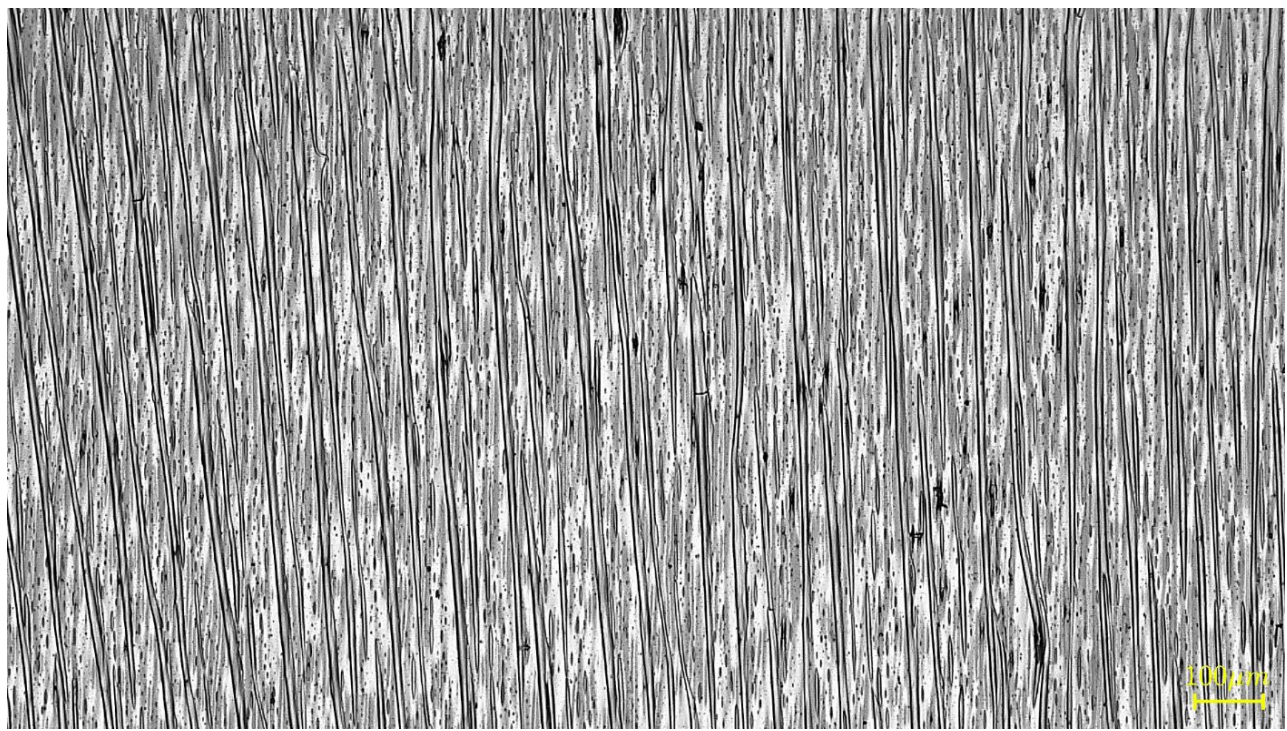

b) Optical microscopy image of polystyrene coated magnetic nanoparticle polystyrene-*b*-polybutadiene matrix formed after solution coating onto a Si wafer in the STVA environmental chamber with an 80% toluene saturated nitrogen atmosphere during drying and with the full array of permanent magnets installed inside the STVA chamber. Inset represents 100 microns.

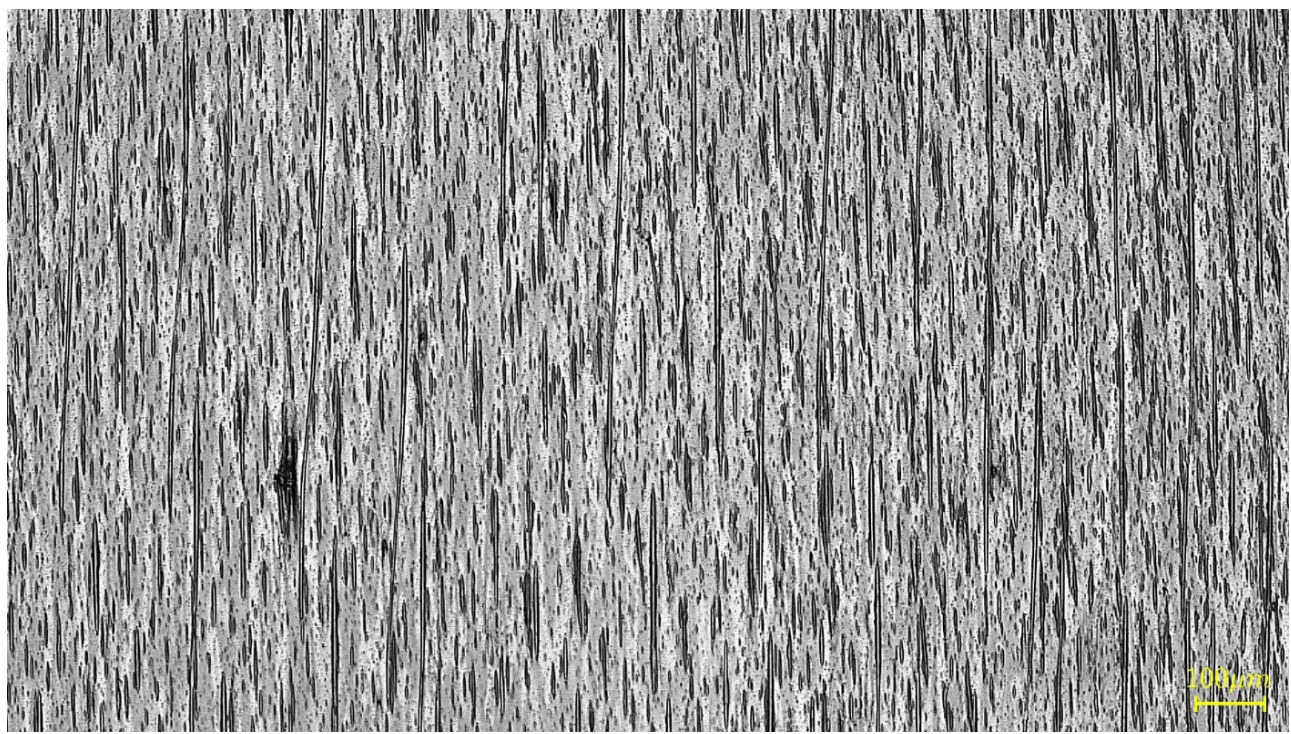

c) Optical microscopy image of polystyrene coated magnetic nanoparticle and block-polymer structure after solution coating onto a Si wafer in the STVA environmental chamber with a toluene saturated nitrogen atmosphere during drying and with no magnets installed inside the STVA chamber. Inset represents 100 microns.

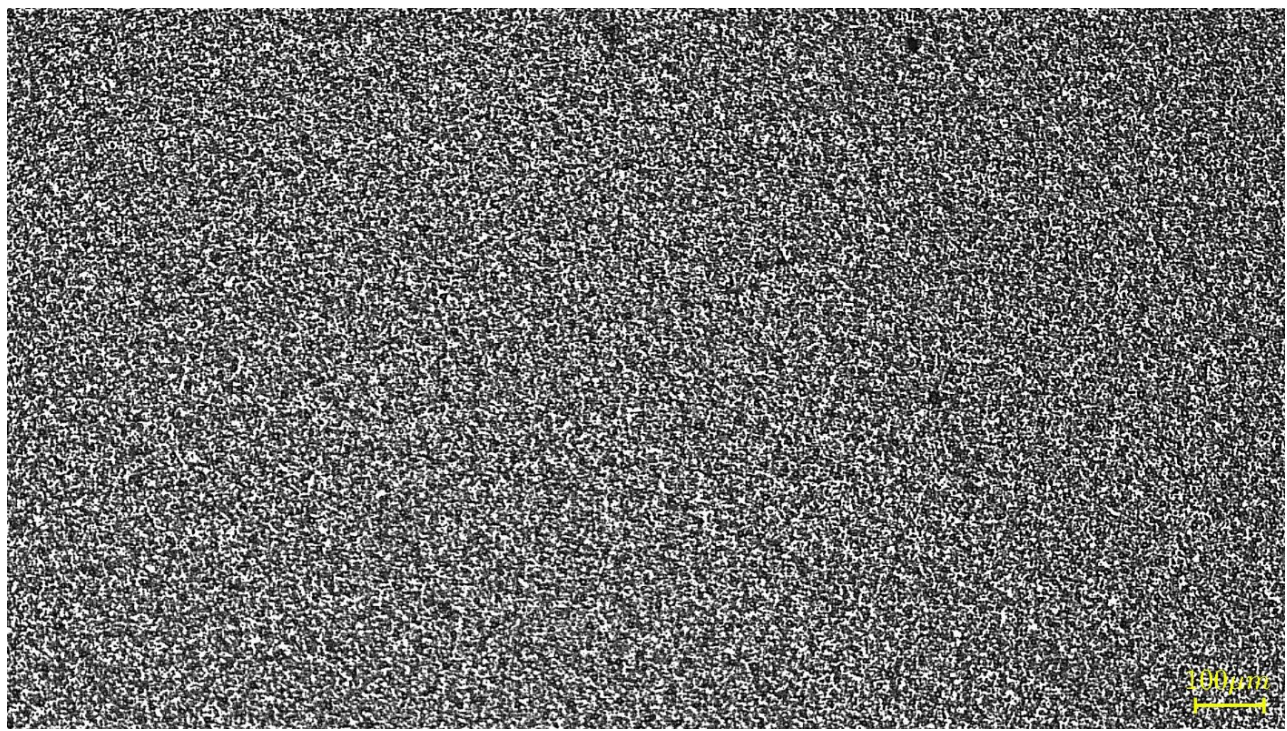

d) Optical microscopy image of polystyrene coated magnetic nanoparticle and polystyrene homopolymer solution on a Si wafer after drying in the STVA environmental chamber with a 80%

toluene saturated nitrogen atmosphere during drying and with the full array of permanent magnets installed inside the STVA chamber. Inset represents 100 microns.

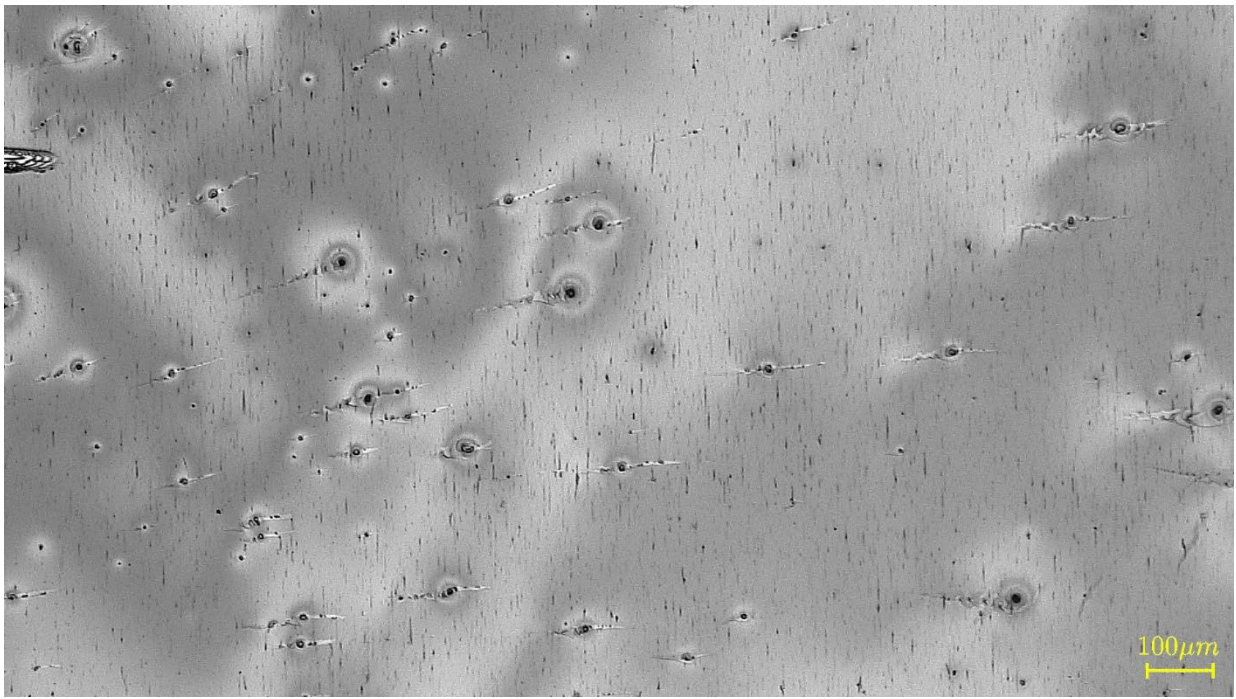

e) Same as d), but with polybutadiene homopolymer instead of polystyrene. The sample shows clear signs of delamination as the nanoparticles segregate from the homopolymer matrix due to immiscibility.

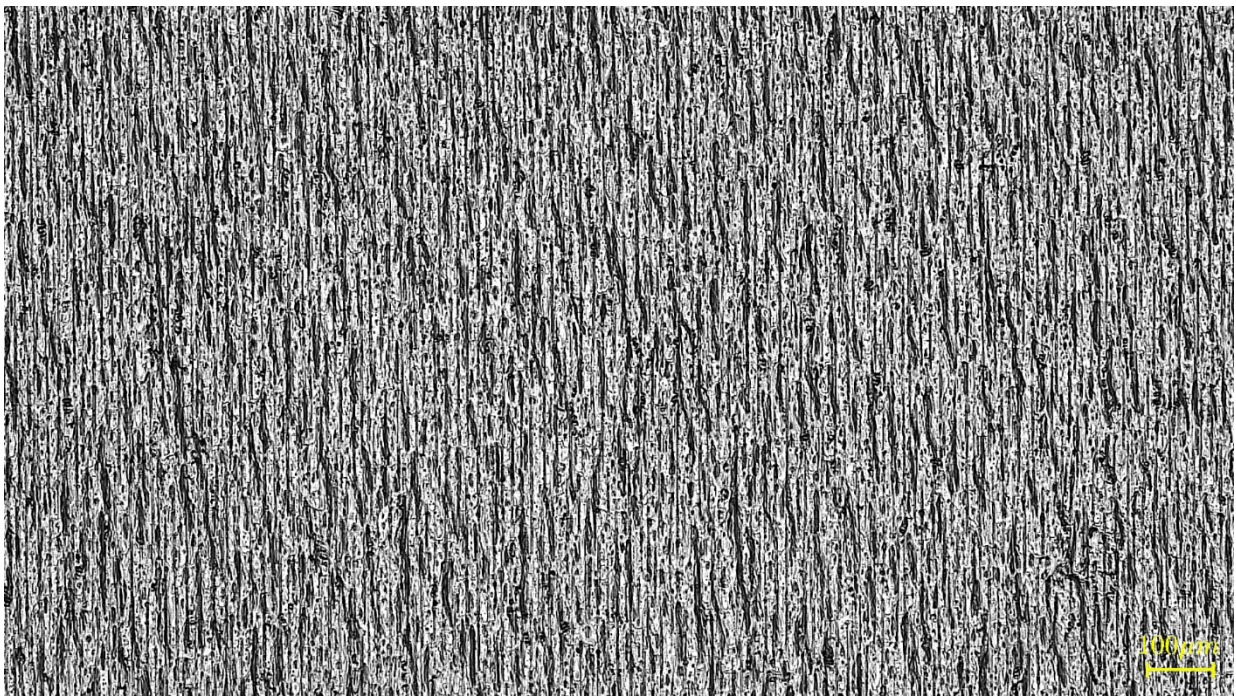

**Figure S6: AFM of PS(38)-*b*-PF2MS(11)**

a) AFM topography maps of polystyrene(38)-*b*-poly(ferrocenyl dimethyl silane)(11) thin films. The samples are annealed in the STVA chamber at toluene humidity levels and temperatures 48% at 35°C (left) and 52% at 25°C (right).

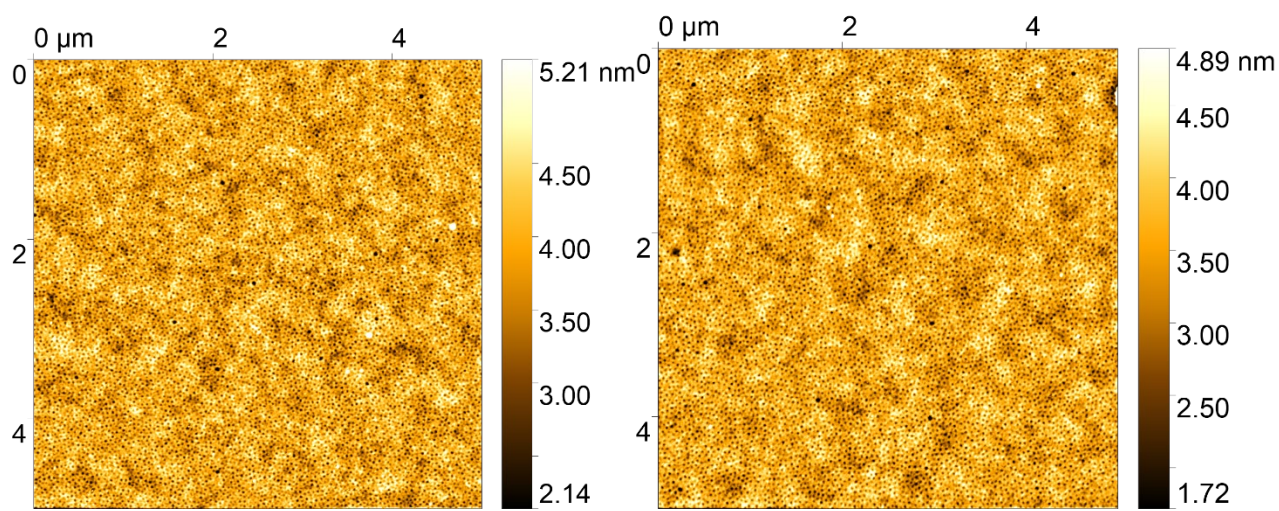

AFM topography map of un-annealed polystyrene(38)-*b*-poly(ferrocenyl dimethyl silane)(11) sample:

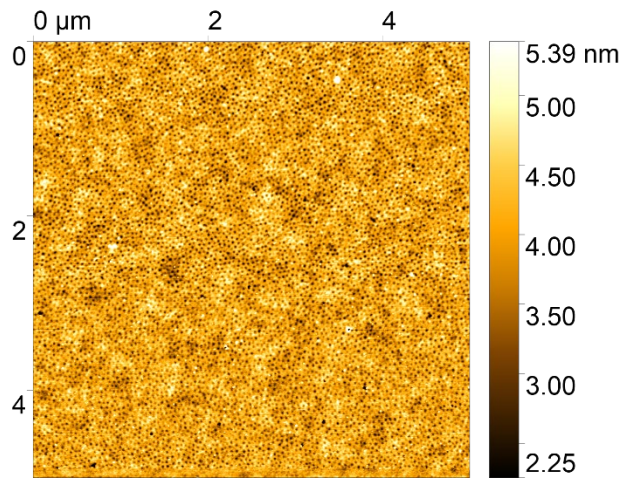

b) 2D Fourier transforms of AFM topography maps of polystyrene(38)-*b*-poly(ferrocenyl dimethyl silane)(11) thin film samples. The samples are annealed in the STVA chamber at toluene humidity levels and temperatures 48% at 35°C (left) and 52% at 25°C (right). Fourier transform of the AFM topography map of the unannealed sample (as spun) is presented in the 3<sup>rd</sup> panel. Radial peaks represented as red lines.

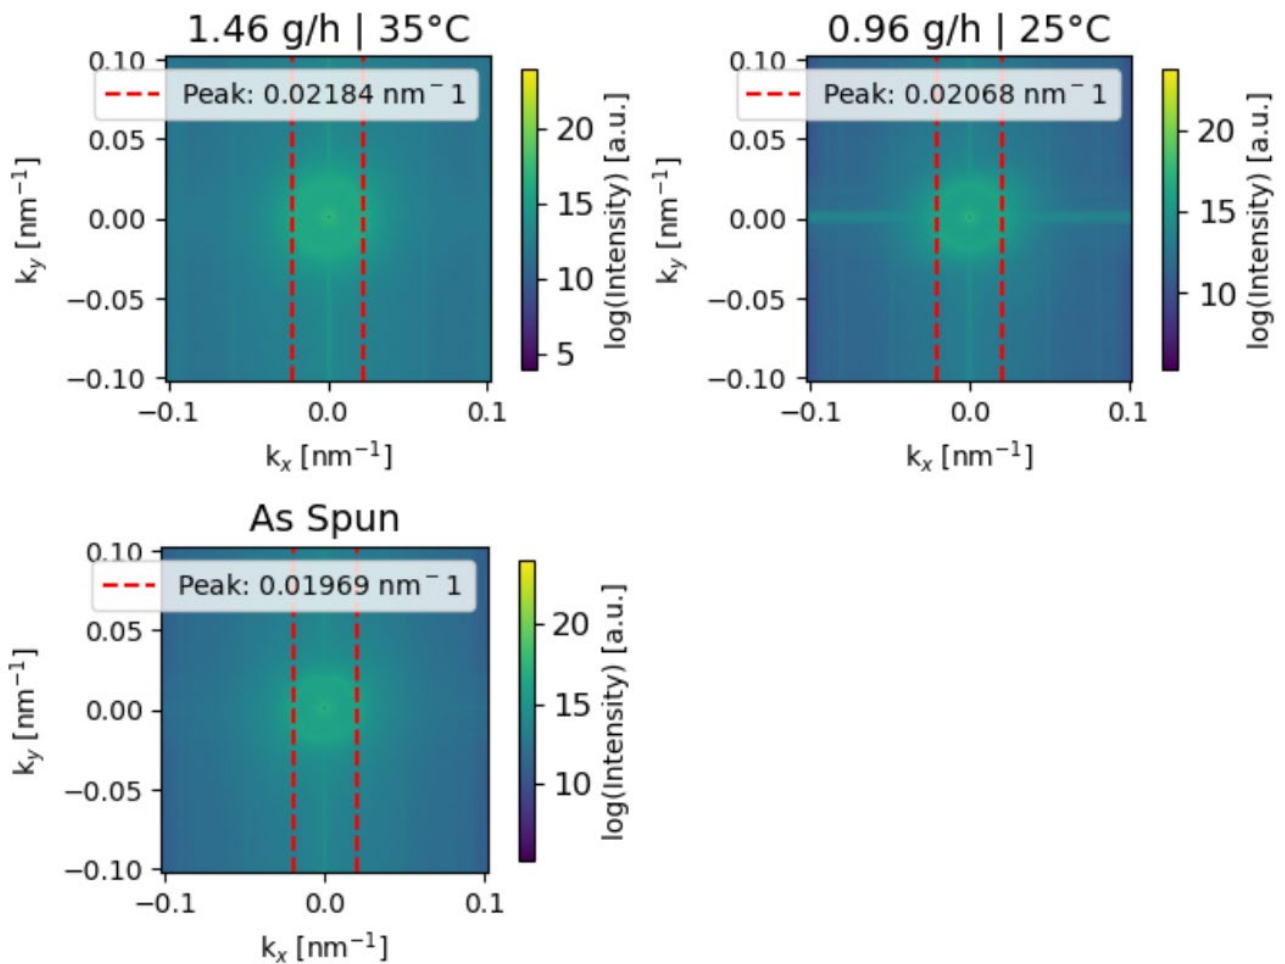

**Figure S7: AFM phase contrast maps of PS(21.7)-*b*-PB(60)**

a) Full size AFM phase contrast maps of polystyrene(21.7)-*b*-polybutadiene(60) thin films, un-annealed (as spun) - top and annealed for 4 hours in 80% toluene saturated nitrogen gas flow – bottom, with associated Fourier transforms of the maps.

As spun:

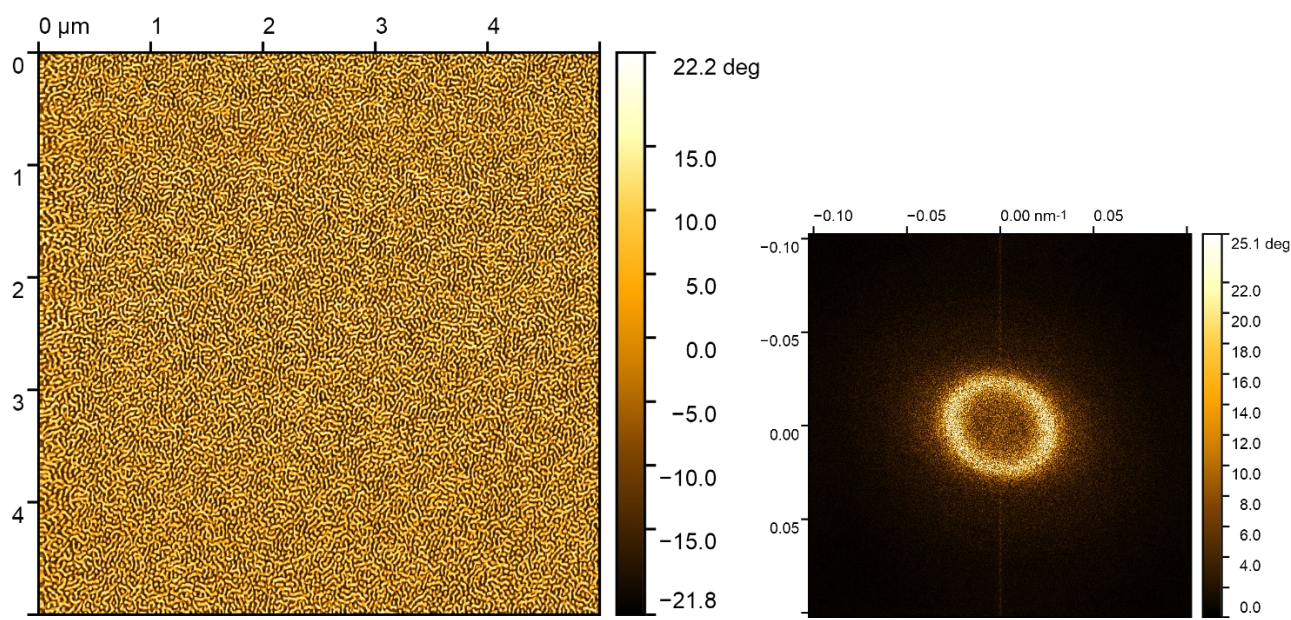

Solvent annealed:

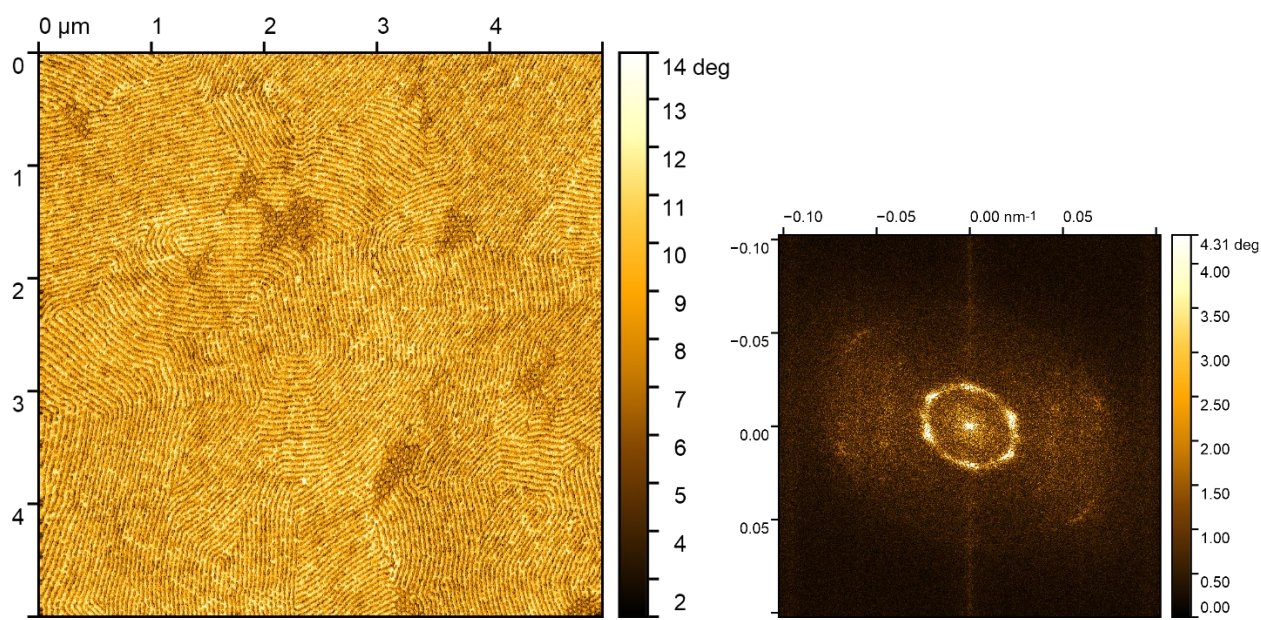

b) 2D Fourier transforms and radial peak positions (red lines) for the two polystyrene(21.7)-*b*-polybutadiene(60) films.:

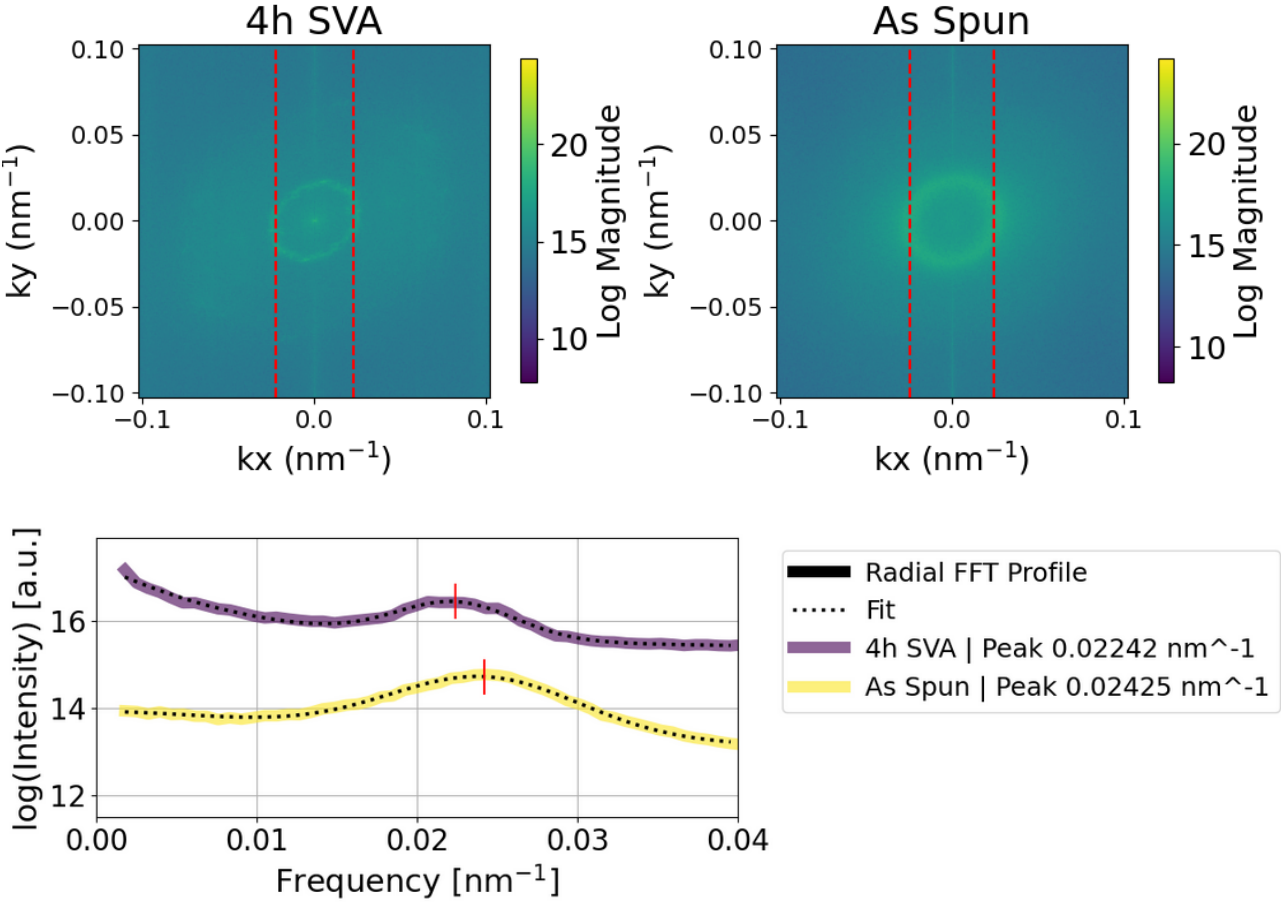

Supplement: Supplementary file 1 [file SupplementaryMaterial.pdf]
